# Supplementary material for: Best-of-Both-Worlds Algorithms for Linear Contextual Bandits
Source: arXiv:2312.15433 source file (2024-02-19)
Supplement: Supplementary file 1 [file appendix_for_experiments.tex]

\section{Details of experimental settings}\label{appendix:experiments}

%\newcommand{\ftr}[0]{\textsc{FTRL-LC}} \YK{we use \algmainFTRL}

% \begin{figure}[ht]
%   \centering

%   \subfigure[Stochastic]{
%     \includegraphics[width=0.3\linewidth]{figure/Stochastic-20-12.pdf}
%     \label{fig:stochastic}
%   }
%   \hfill
%   \subfigure[Stochastic with adversarial corruptions]{
%     \includegraphics[width=0.3\linewidth]{figure/Corrupted-20-12.pdf}
%     \label{fig:corrupted}
%   }
%   \subfigure[Stochastic phase]{
%     \includegraphics[width=0.3\linewidth]{figure/Phase-20-12.pdf}
%     \label{fig:phase}
%   }
%   \caption{Average pseudo regret obtained after $10^5$ time steps over 35 runs in the three environment settings described.}
%   \label{fig:mainfigure}
% \end{figure}
% \begin{figure}
%     \centering
%     \includegraphics{figure/Stochastic-20-12.pdf}
%     \caption{Caption}
%     \label{fig:enter-label}
% \end{figure}

We experimentally evaluated the performance of \algmainFTRL\ by comparing it with two baselines, specifically designed for the stochastic or the adversarial setting. We implemented the \textsc{OFUL} algorithm by \cite{abbasi2011improved} as the stochastic baseline and \textsc{LinExp} by \cite{neu2020efficient} for the adversarial setting.
We now describe

\paragraph{Context generation} In order to generate the contexts from a fixed distribution, we employed two different techniques:
\begin{itemize}
    \item \textbf{Uniform}: A fixed number of contexts $X_t \in \mathbb{R}^{d}$ are generated, where for each $i \in [d]$, $X_t(i)$ is drawn from a normal distribution with a mean of zero and a variance of $0.3$. These contexts are then normalized such that $\| X_t\|_2 = 1$. One of these contexts is selected uniformly at random to serve as the current context.
    \item \textbf{Normal}: The current context $X_t \in \mathbb{R}^{d}$ is generated such that for each $i \in [d]$, $X_t(i)$ is drawn from a normal distribution with zero mean and a variance of $0.3$. It is then normalized to ensure $\| X_t\|_2 = 1$.
\end{itemize}

The reward settings are currently three:

\begin{itemize}
    \item \textbf{Stochastic}: a $\bm{\theta}_a \in \R^{d}$ vector is selected for each action $a \in [K]$. For all $i \in [d]$, each $\theta^i_{a}$ is drawn from a normal distribution with zero mean and unit variance and then is normalized in order to set $\| \bm{\theta_a}\|_2 = 1$. Each time an action $a \in [K]$ is selected, the loss obtained is equal to $\la \bm{\theta_{a}}, X_t \ra + \epsilon_t$ with $\epsilon_t \sim N(0,0.3)$.
    %To ensure the loss falls in the $[-1,1]$ interval, it is clipped.
    
    \item \textbf{Stochastic with adversarial corruptions}.
    Here the reward schema is the same as before, but there is a corruption parameter (set to $\sqrt{T}$), such that for the first $\sqrt{T}$ time steps the loss will be $-\la \bm{\theta_{a}}, X_t \ra + \epsilon_t$ with $\epsilon_t \sim N(0,0.3)$.
    
    \item \textbf{Stochastic phase}. This setting is inspired by the experimental configuration of \cite{ZimmertSeldin2021}. The environment alternates between two stochastic configurations. In the first configuration, the optimal arm has an expected loss of 0, while the sub-optimal arms have an expected loss of $0.125$. In the second configuration, the expected losses for the arms are $1 - 0.125$ and $1$, respectively. 
    The transition between these two settings occurs at intervals that increase exponentially by a factor of $1.6$. 
\end{itemize}

In all of these settings, in order to ensure that the loss falls within the $[-1,1]$ interval without affecting the distribution used to generate the noise, a procedure of rejection sampling is adopted.

\YK{Since $\beta_t$ is already used to define $\eta_t$, crucial quantity, could you use another notation here? Maybe, meaning confidence radius, can we use $\mathrm{rad}_t$ instead of $\beta_t$?}
I attach the implementation of the \textsc{OFUL} algorithm in order to show either the way I am using to compute the covariance matrix of the contexts and to actually implement this algorithm in a ``policy" way: 
\begin{enumerate}
    \item \textbf{Initialize:} 
    
    \begin{enumerate}
        \item covariance tensor $\mathfrak{C} \in \R^{K \times d \times d}$. For each row (action) set $\lambda I \in \R^{d \times d}$ with $\lambda$ regularization hyperparameter (only for \textsc{OFUL} is different from 0).  \YK{$\lambda$ should be specified}
        
        \item Initialize also the cumulative loss matrix $B \in \R^{K \times d}$. Each row (action) as $\bf{0} \in \R^{d}$.
        \item Initialize the $\hat{\bf{\theta}}_a = \bf{0} \in \R^{d}$ for each action $a \in [K]$.
    \end{enumerate} 
    
    \item \textbf{Predict}($X_t$): return $\argmin_{a \in [k]} \la \hat{\bf{\theta}}_a, X_t \ra - \beta_t \| X_t\|_{\Sigma^{\dag}_{t,a}}$,~ where $\beta_t = \sqrt{d\ln{\frac{1 + t/\lambda}{\delta}}} + \sqrt{\lambda}$ and $\delta \in (0,1)$\YK{We should compute confidence ellipsoids in \citet{abbasi2011improved}}
    
    \item \textbf{Update}($X_t$, $A_t$, $\ell(X_t, A_t)$):\YK{$\ell$ is undefined. Here $\ell,a$ should be $\ell_t(X_t, A_t)$ and $A_t$?}
    \begin{enumerate}
        \item update covariance tensor $\mathfrak{C}_{A_t}= \mathfrak{C}_{A_t} + X_tX_t^T$.  \YK{It would be better to define those statistics with each round $t$. $X$ should be $X_t$?}
        \item update $B_{A_t} = B_{A_t} + \ell(X_t, A_t) X_t$
        \item update $\hat{\bf{\theta}}_{A_t} = \mathfrak{C}^\dag_{A_t} B_{A_t}$
    \end{enumerate}

\end{enumerate}
